# Supplementary material for: Non-Autoregressive Electron Redistribution Modeling for Reaction Prediction
Source: arXiv:2106.07801 source file (2021-06-08)
Supplement: Supplementary file 2 [file 6-appendix.tex]

\newpage

\section{Appendix A: Controllability and Interpretability of Latent Variable.}
We figure out some directions in latent space of $z$, denoted by a vector $v$, to indicate corresponding polarity properties of predicted molecules. For example, in figure~\ref{Redox-S} we sample latent $z$ from multiplies of $v$, where the factors are in a subset, here $\{-8,-4,-2,-1,0,1,2,4,8\}$. The factors for our predictions in order is $ a: -4, -2, -1, 0, 1, b:2, c:4$. \\
The direction $v$ is computed by the polarity concerning the addition and subtraction of total edge weight among the product atoms, and the atoms in the product is provided by ground truth. The resulting direction is consistent with the reduction and oxidation tendency in the chemical principle.\\

Therefore, our NERF with latent variable is feasible for chemists to interpret multimodal outputs, reflecting domain knowledge learned automatically. Furthermore, assuming uncertainty of product prediction partially comes from various chemical conditions or environments, controlling latent $z$ may augment the NERF model with additional guidance and boost its performance, like grid search in the latent space instead of just change temperatures, especially in the real world settings.\\
Figure~\ref{Redox-O} (c) is an exception, the atoms inside the product graph form a ring, which is consistent with our graph theory measure, yet not with chemical assumption.

\begin{figure*}[t]
        \centering
        \includegraphics[width = 0.8\linewidth]{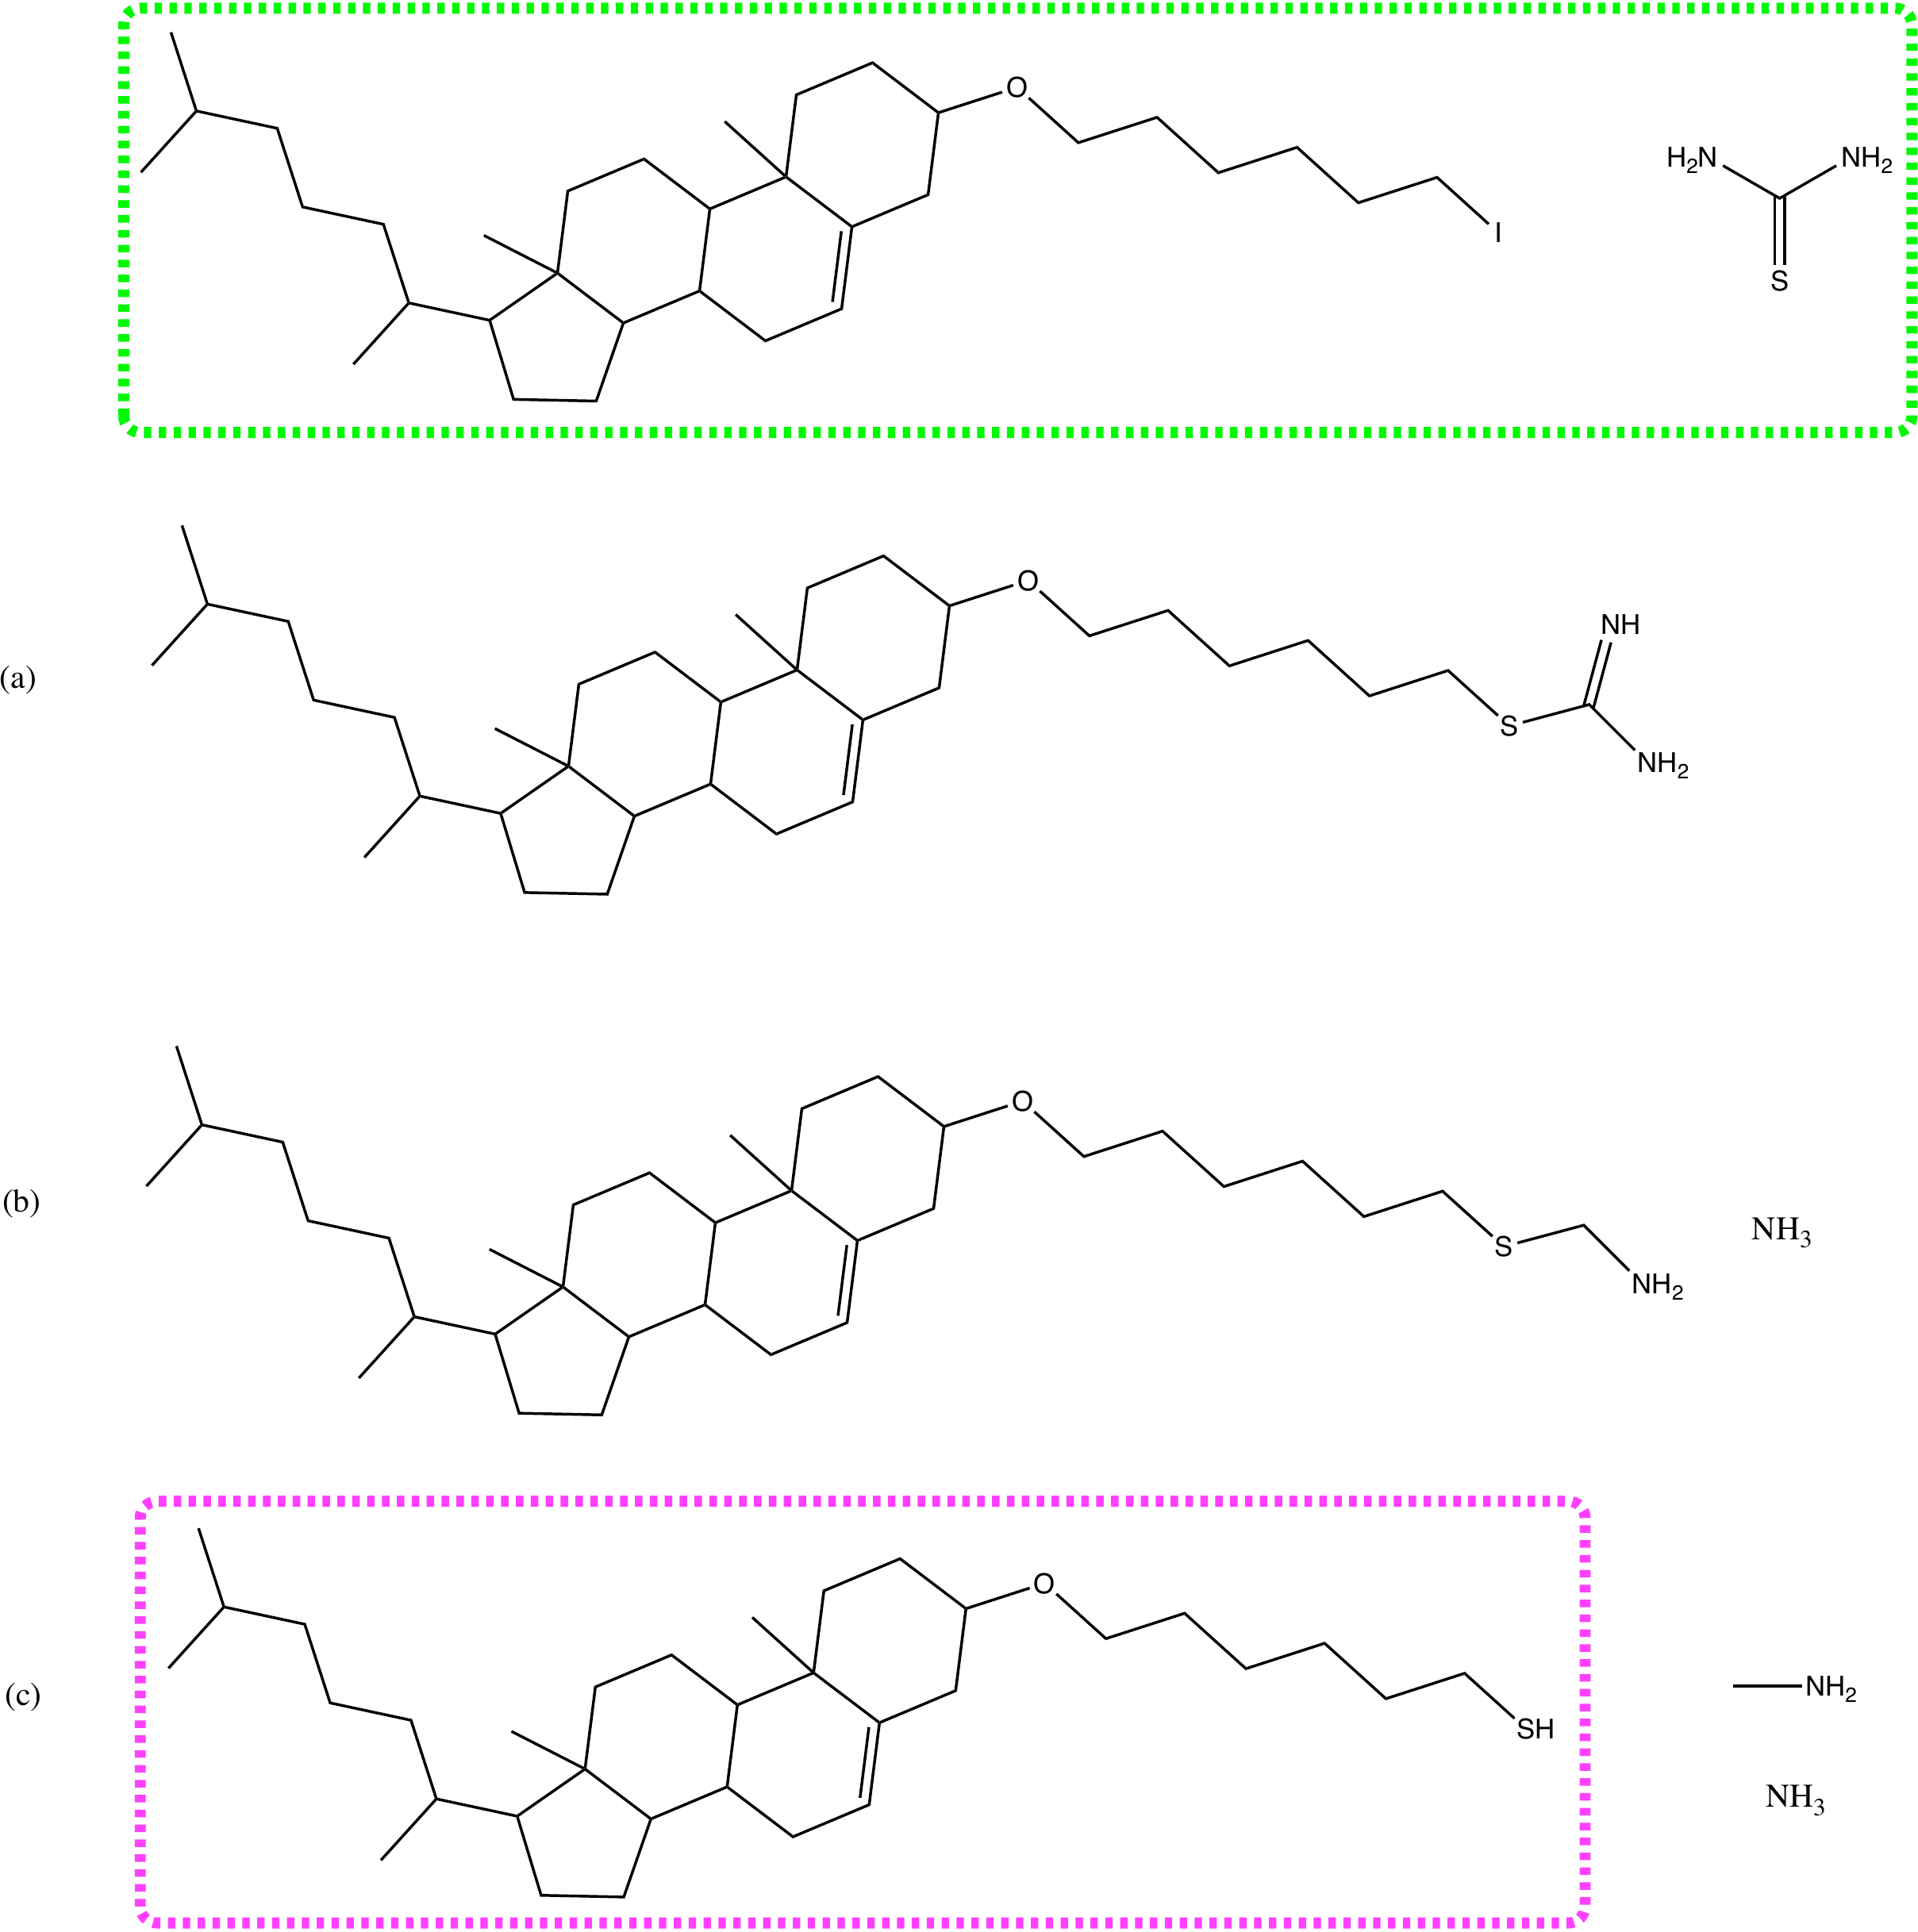}
       % \caption{Product outcomes  generated by  NEFG. The electron flow on the reactants is predicted via a conditional variational encoder-decoder framework.         }
       \caption{controllable prediction of a Redox reaction. The molecules in the green box is the reactants, and (a) (b) (c)  the output of our NERF. The generation is controlled by the direction in latent space w.r.t. bond counts in the product segment, which is in the purple box. We omit some trivial reactants and byproducts, such as $H_2O$.}
        \label{Redox-S}
\end{figure*}	

\begin{figure*}[t]
        \centering
        \includegraphics[width = 0.8\linewidth]{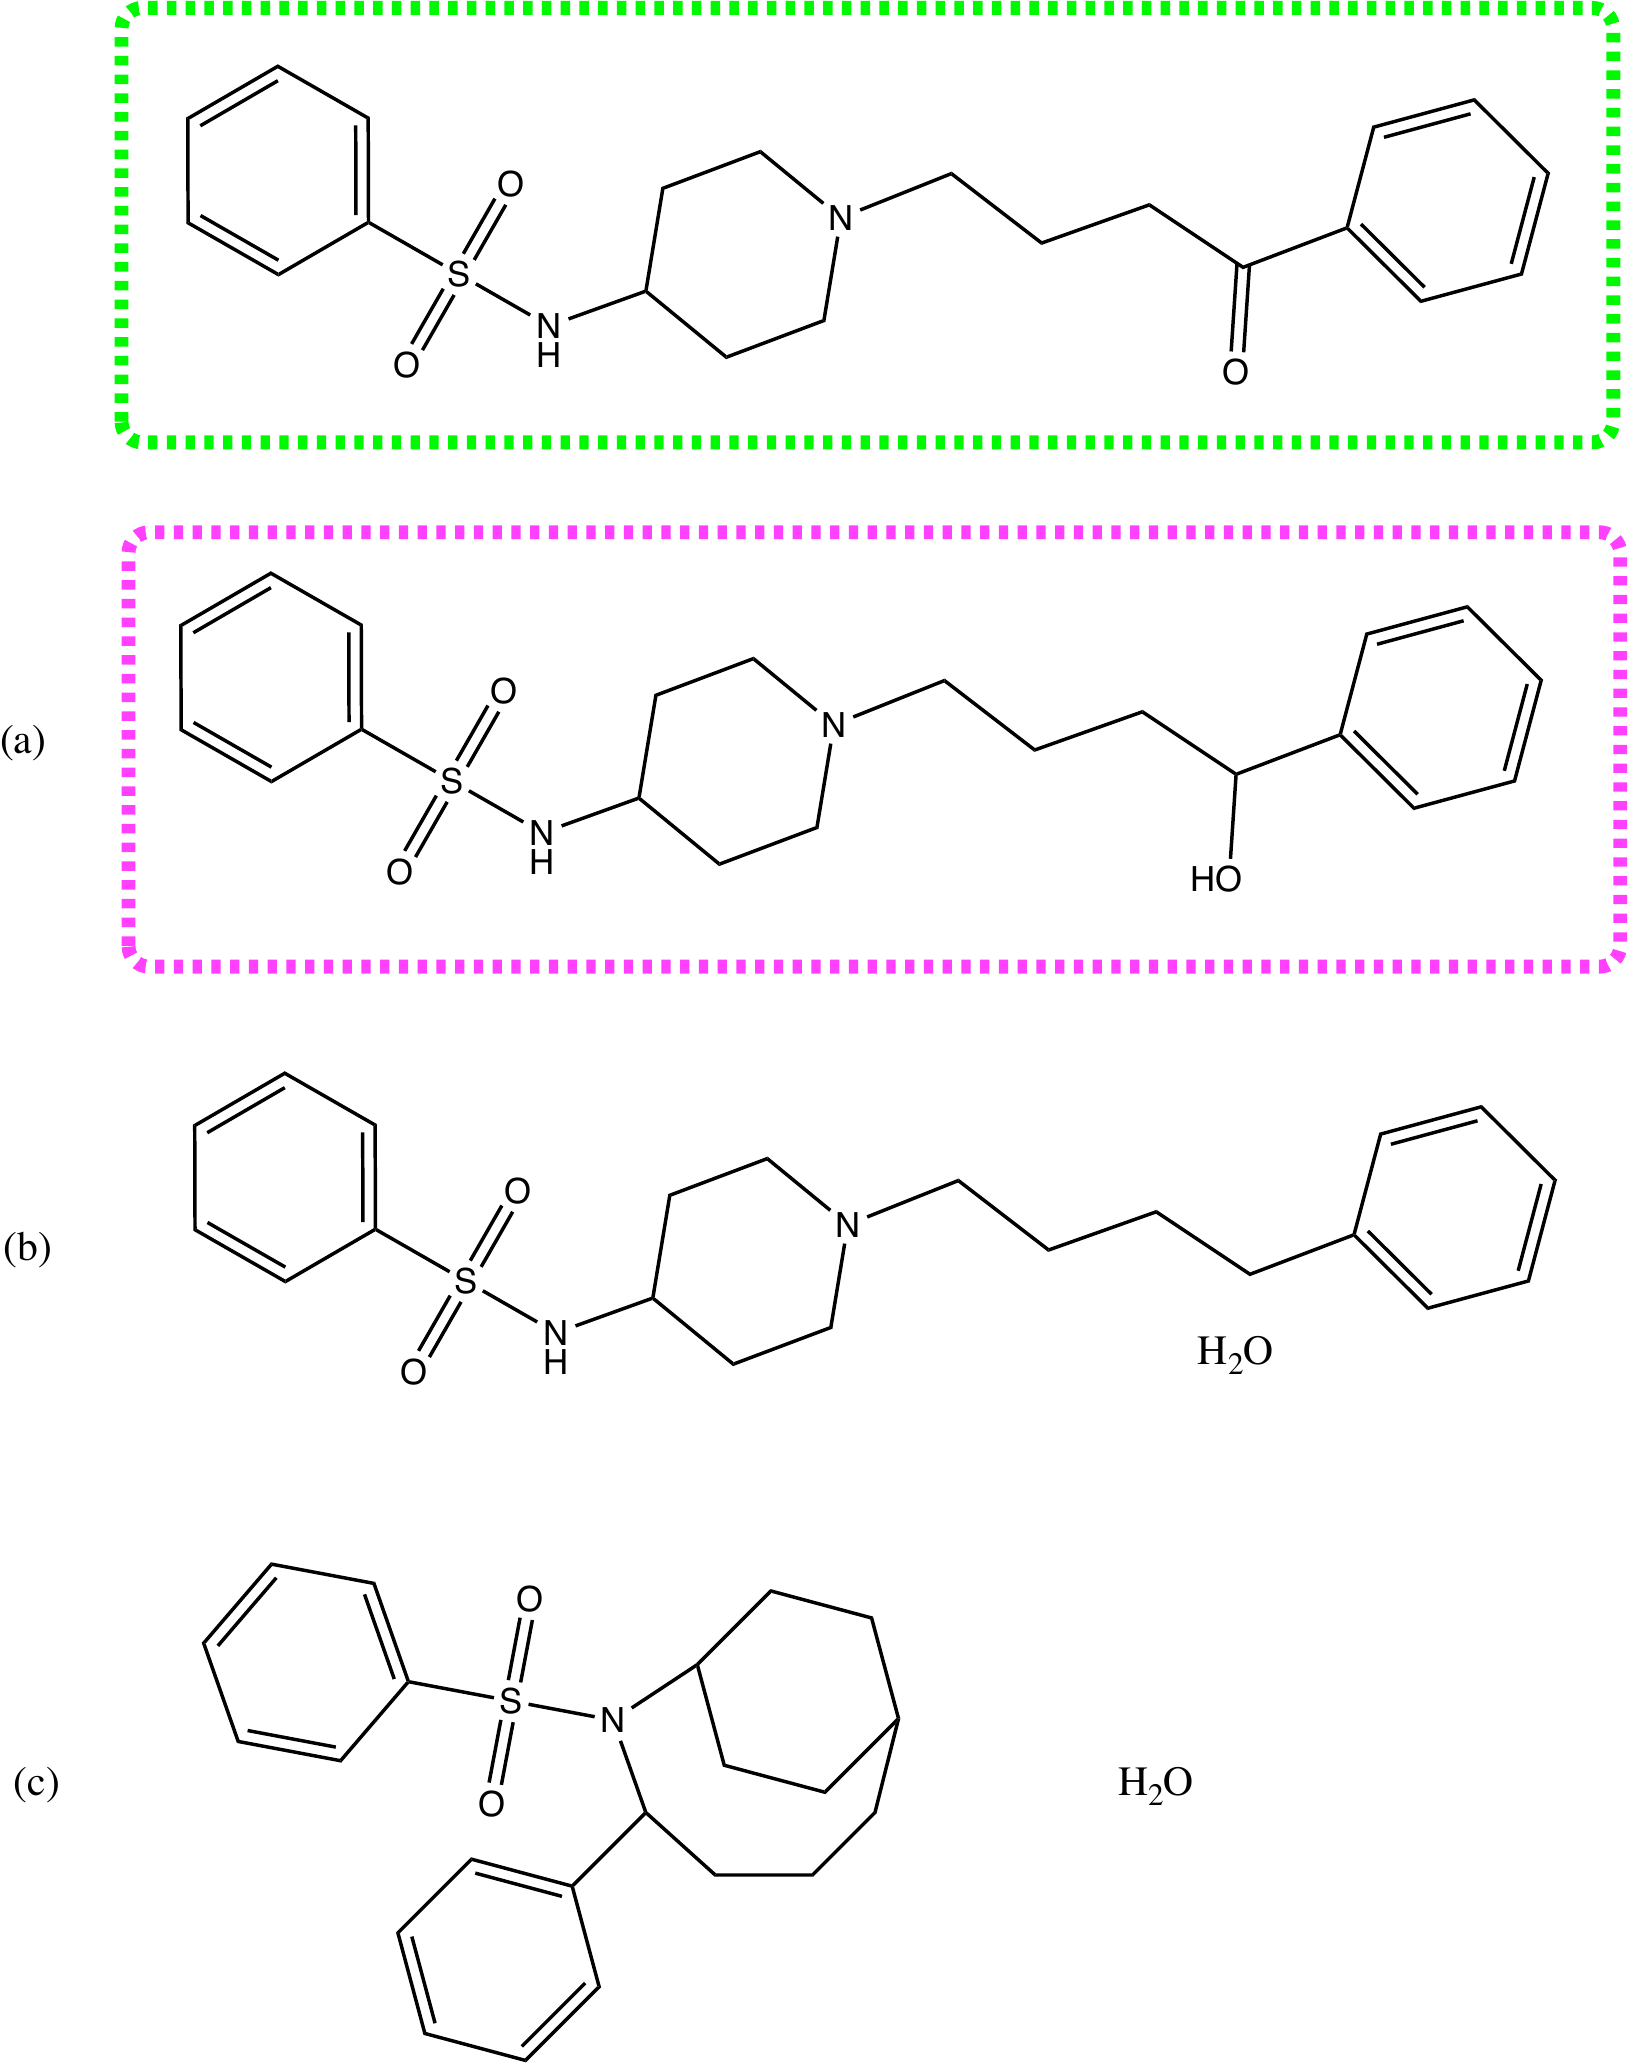}
       % \caption{Product outcomes  generated by  NEFG. The electron flow on the reactants is predicted via a conditional variational encoder-decoder framework.         }
       \caption{controllable prediction of a Redox reaction. The molecules in the green box is the reactants, and (a)-[-8,-4,-2,-1] (b)-[0] (c)-[1,2,4,8]  the output of our NERF. The generation is controlled by the direction in latent space w.r.t. bond counts in the product segment, which is in the purple box.}
        \label{Redox-O}
\end{figure*}	

\HB{figure 5, b to d is nice. Indicating the size of the product or degree of oxidation. We need a table.}

\HB{Table x shows our results for manipulating the VAE output by extrapolating vectors in the latent space. 
1. We identify some Boolean features (e.g. if the product is larger than all reactants, or if the reaction topology is linear).
2. For a certain feature, we find all positive samples in the test set that have such feature.
3. Take the average of all latent vectors of positive samples, $\bm{v}$, which we assume is the hidden dimension that encodes such feature.
4. For all samples in the test set, we set the latent vector to $\alpha \bm{v}$, where alpha ranges from -8 to +8. We record for each alpha the percentage of predictions that are positive in the feature.
}
\HB{Do remember to cite a VAE article in CV, which used the same interpretation method}

property: edge weight in product graph:\\
8  20.5 \\
4  21.5 \\
2  19.7 \\
1  17.4 \\
0  14.0 \\
-1 9.5 \\
-2 8.4 \\
-4 6.8 \\
-8 5.3 \\
\section{Appendix B: Reaction Topology Illustration}

Here we provide more examples to show our three representative topology and our model prediction.

\begin{figure*}[t]
        \centering
        \includegraphics[width = 1.0\linewidth]{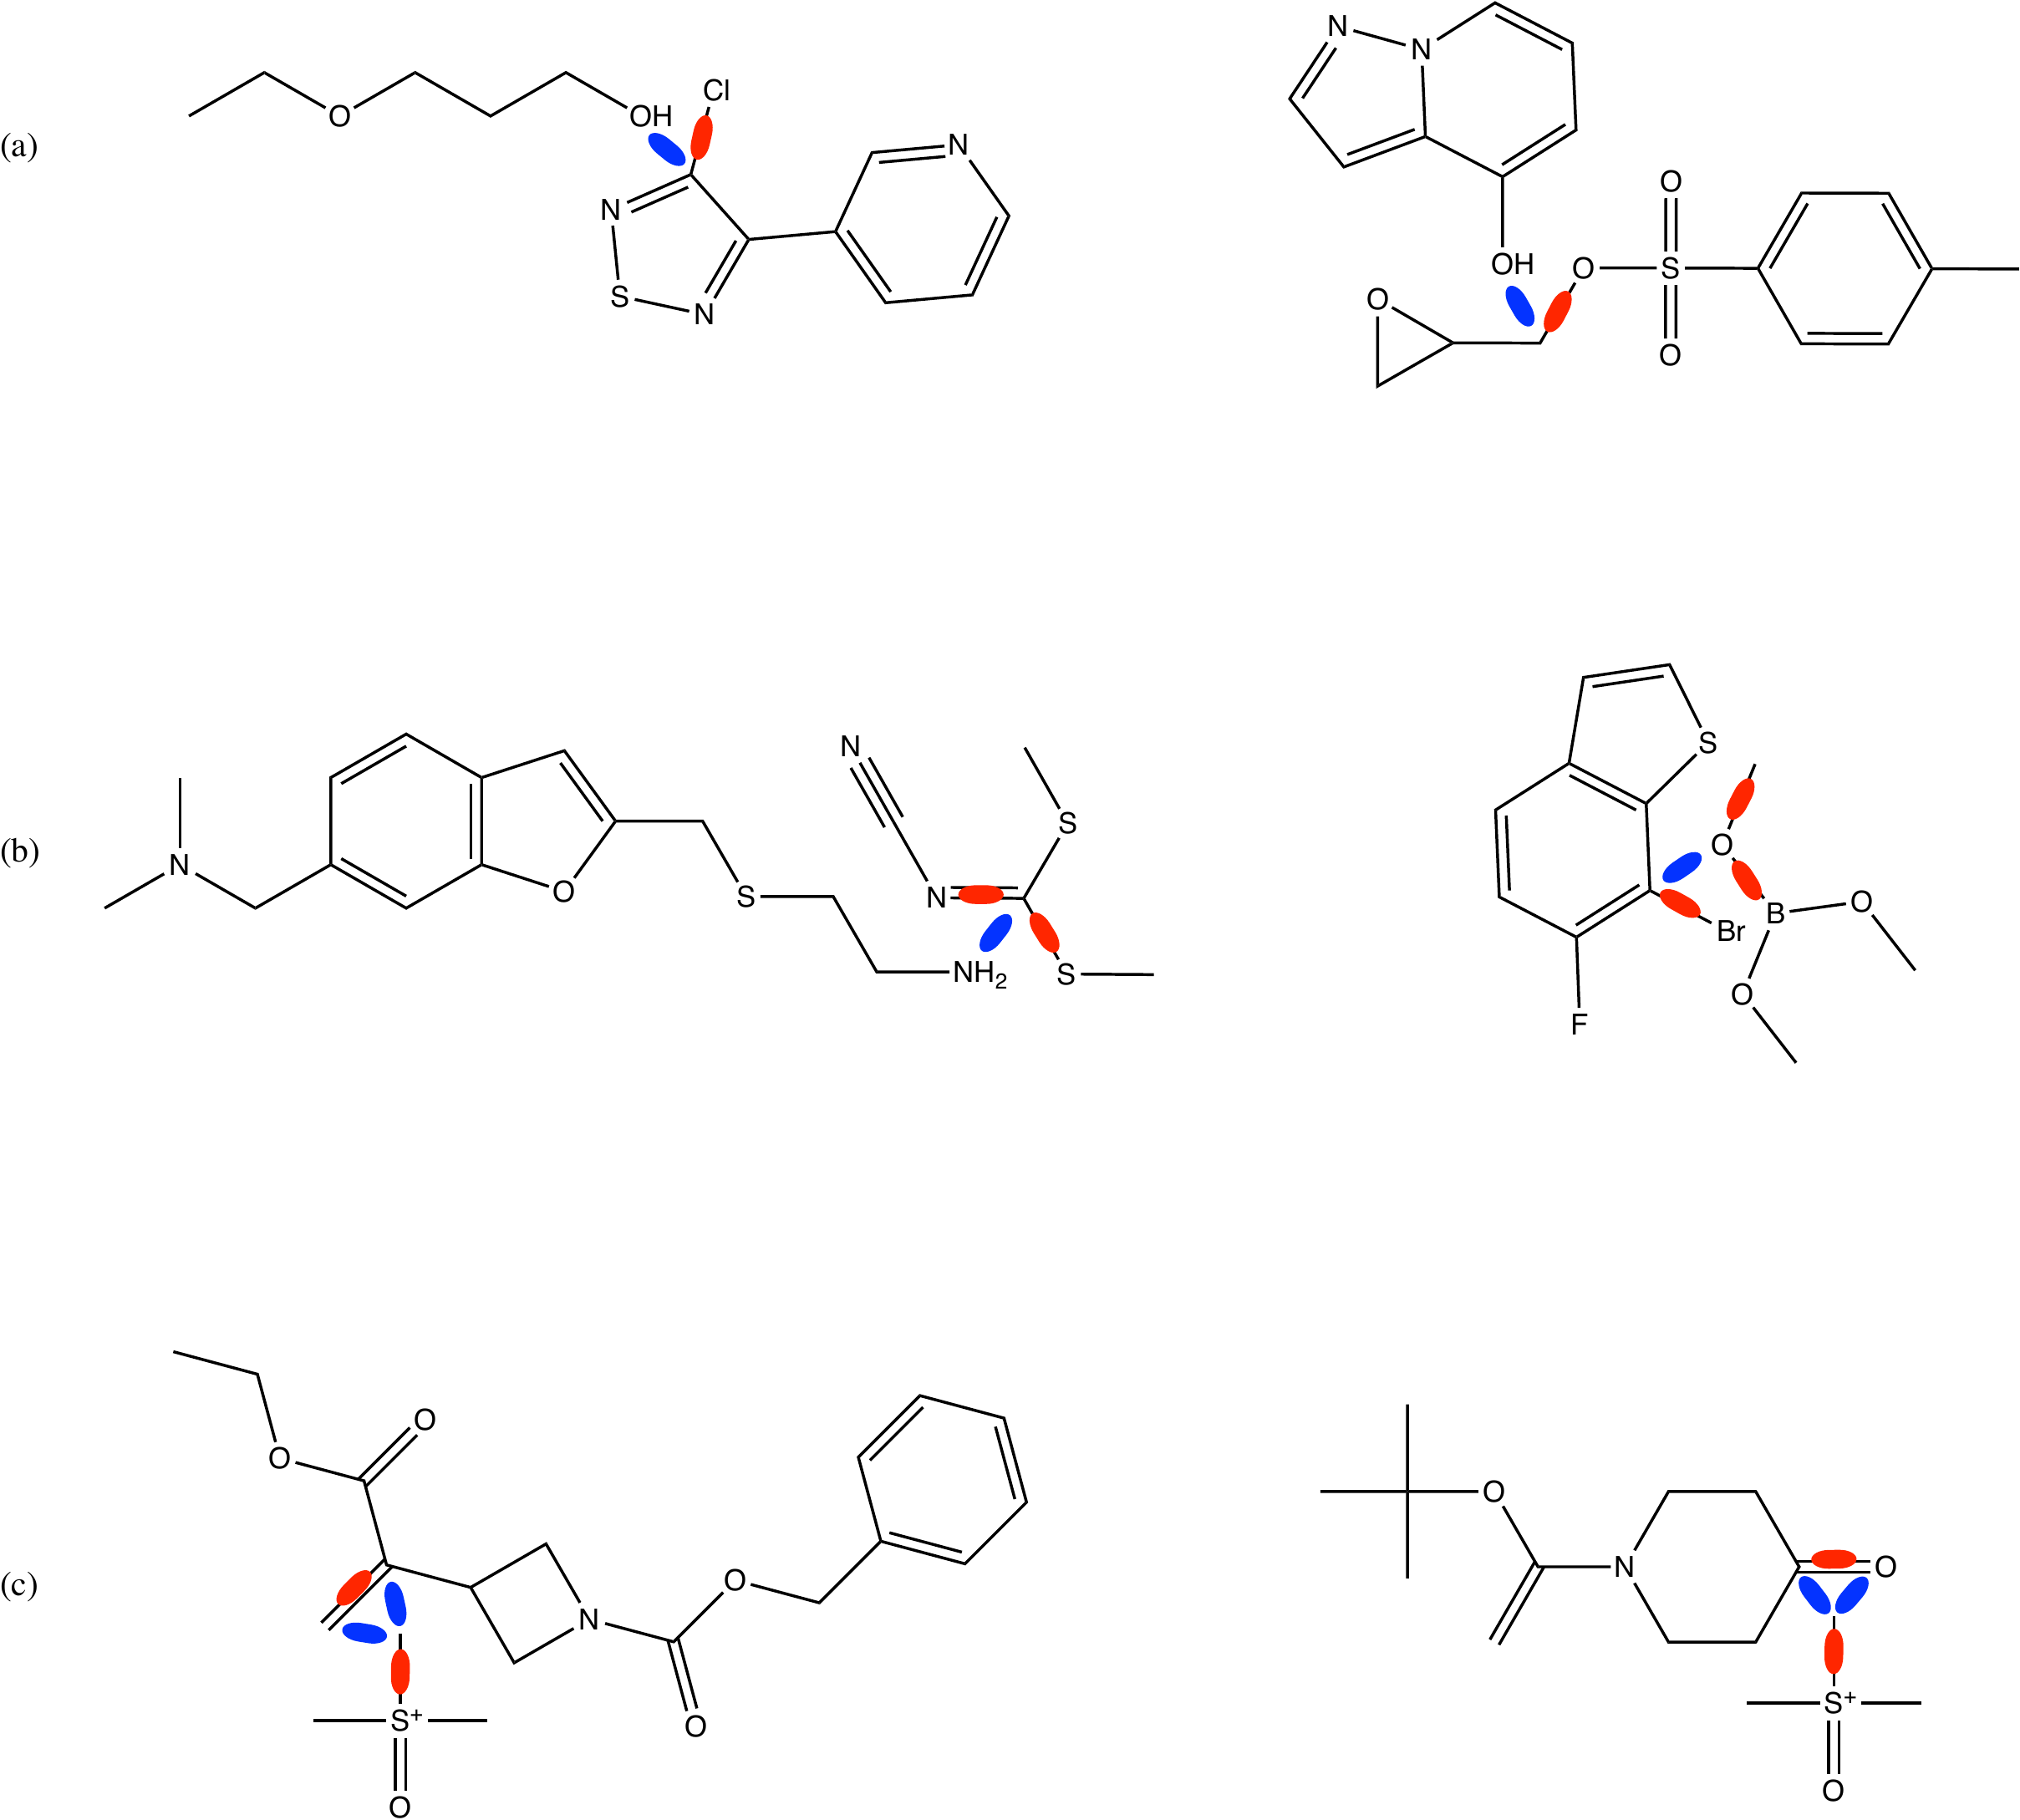}
       % \caption{Product outcomes  generated by  NEFG. The electron flow on the reactants is predicted via a conditional variational encoder-decoder framework.         }
       \caption{(a)(b)(c) are samples of reaction centers~\cite{WLN2017jin} in linear, branch, and cyclic topology respectively.}
        \label{topology+}
\end{figure*}
